# Supplementary material for: Magnetotransport in Sr3PbO antiperovskite with three-dimensional massive Dirac electrons
Source: arXiv:1807.08006 ancillary file (2018-07-20)
Supplement: Supplementary file 1 [file Supplemental.pdf]

# Supplementary Materials for Magnetotransport in $Sr_3PbO$ antiperovskite with three-dimensional massive Dirac electrons

S. Suetsugu[1], K. Hayama[1], A. W. Rost[2,3], J. Nuss[3], C. Mühle[3], J. Kim[3], K. Kitagawa[1] and H. Takagi[1,2,3]

*[1]Department of Physics, The University of Tokyo, 7-3-1 Hongo, Bunkyo-ku, Tokyo 113-0033, Japan.*
*[2]Institute for Functional Matter and Quantum Technologies, University of Stuttgart, Pfaffenwaldring 57, 70550 Stuttgart, Germany.*
*[3]Max Planck Institute for Solid State Research, Heisenbergstrasse 1, 70569 Stuttgart, Germany.*

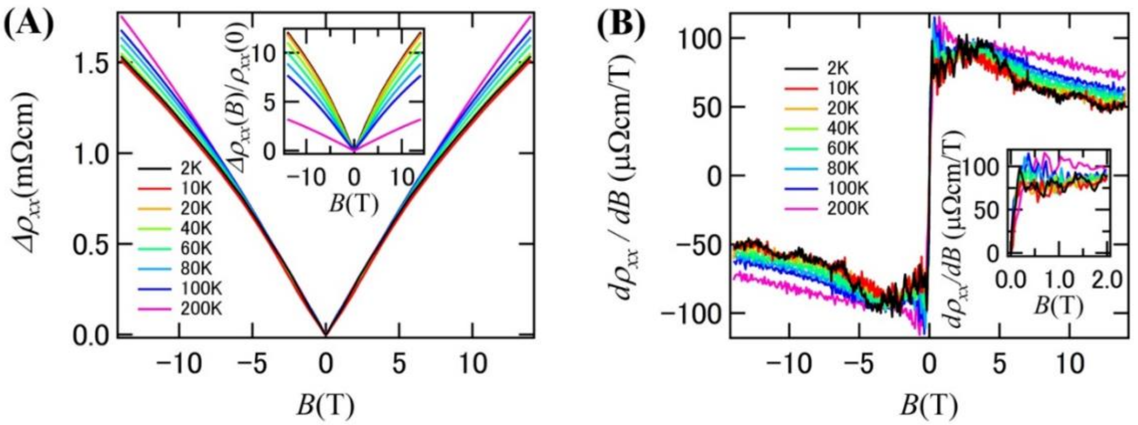


FIG. S1. Magnetoresistance of a single crystal of $Sr_3PbO$ different from the crystal described in the main text.
(A) At $T$ = 2 K, the large MR ratio of over 10 at $B$ = 14 T is reproducibly observed as seen in the inset. Magnetic field dependence of $\Delta\rho_{xx}(B) = \rho_{xx}(B) - \rho_{xx}(0)$ is almost $B$-linear at high fields. (B) Almost $B$-linear behavior of $\Delta\rho_{xx}$ at high field is better visualized in almost $T$-independent and constant derivative of resistivity $d\rho_{xx}/dB$ at least up to 100 K. Low field $T$-independent $B^2$ behavior of $\Delta\rho_{xx}$ is demonstrated by almost $B$-linear behavior of $d\rho_{xx}/dB$ as seen in the inset. The crossover from $B^2$ to $B$ behavior of $\Delta\rho_{xx}$ in this single crystal qualitatively reproduced the results shown in Fig. 3B. The details of field and temperature dependence is slightly different, which may be attributed to the deviation of crystallographic axis against the direction of magnetic field.

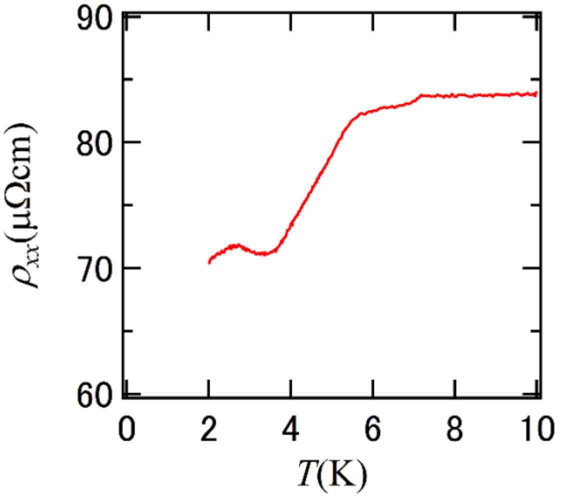


FIG. S2. Filamentary superconductivity of $Sr_3PbO$.
The single crystals of $Sr_3PbO$ from the same batch as the crystal in Figs. 1-4 often showed a resistance drop of up to ~ 10% at low temperatures, indicative of filamentary superconductivity. Zero resistance was never observed down to 2 K.

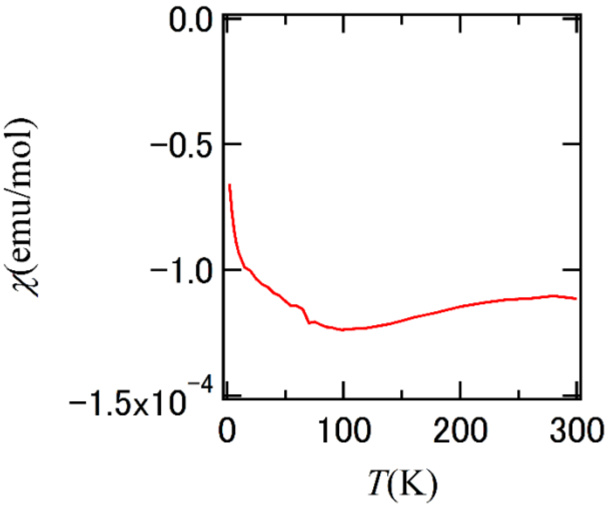


FIG. S3. Magnetic susceptibility of $Sr_3PbO$.
Temperature dependence of magnetic susceptibility $\chi(T)$ of powder sample of $Sr_3PbO$ measured at 1 T. $\chi(T)$ remains diamagnetic and no trace of magnetic transition is observed. This eliminates a magnetic origin of the nonlinear behavior of $\rho_{xy}(B)$.

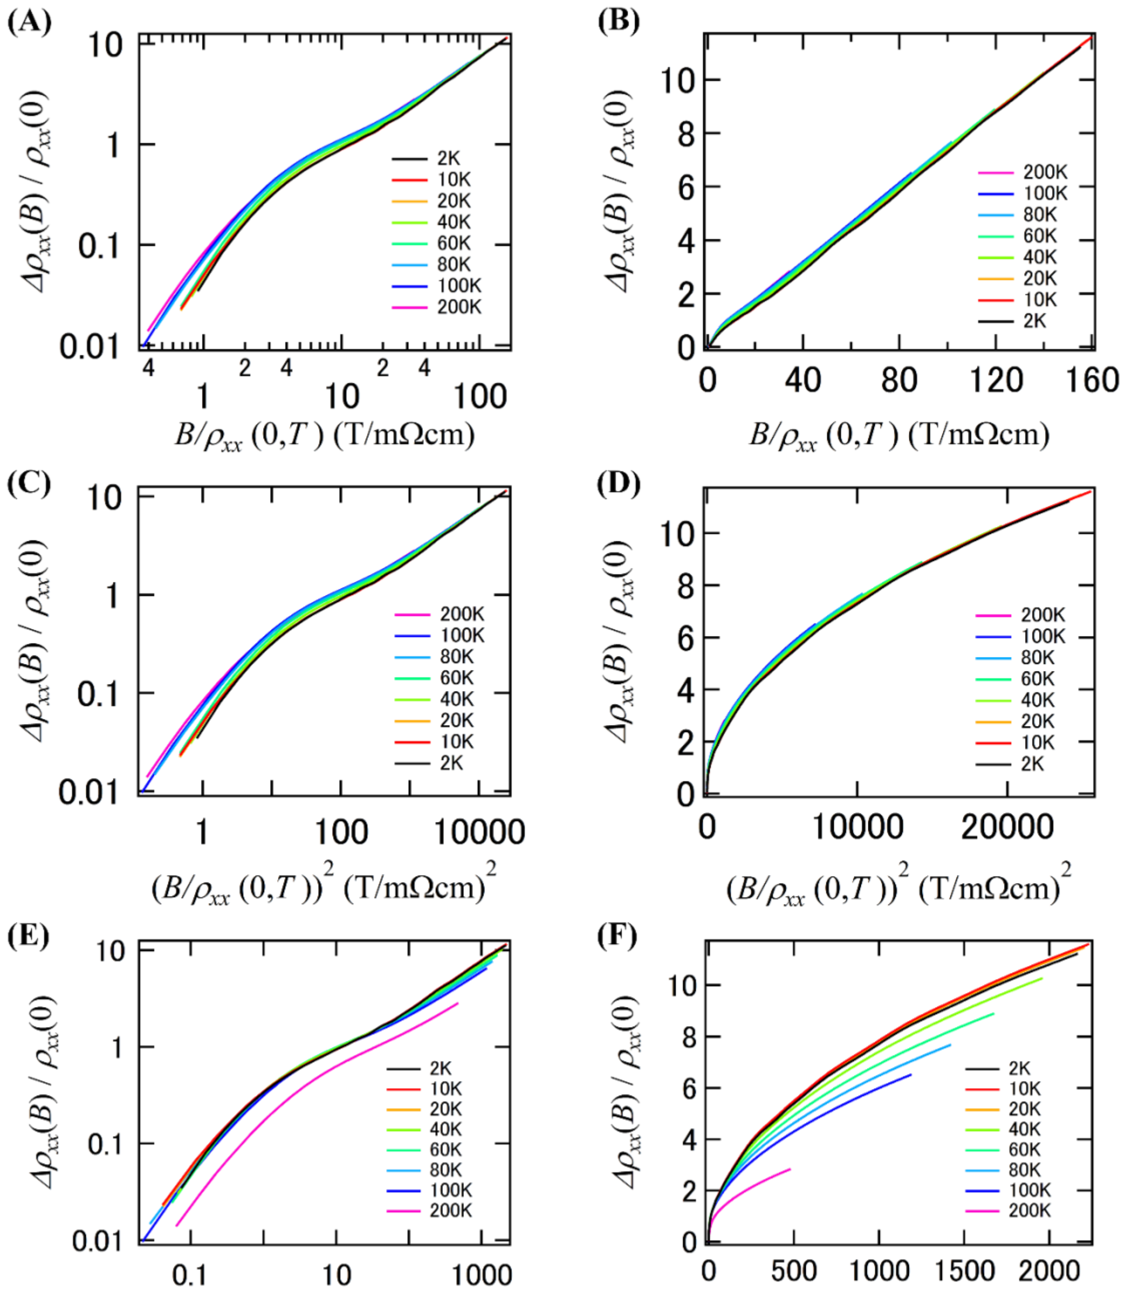


FIG. S4. Scaling plots of magnetoresistance for $Sr_3PbO$ single crystal.
(A-D) $\Delta\rho_{xx}(B,T)/\rho_{xx}(0,T)$ in Fig. 3A is plotted as a function of $B/\rho_{xx}(0,T)$ or $(B/\rho_{xx}(0,T))^2$ using log-log or linear scales. All the curves for different temperatures overlay each other in the high field $B$-linear region but not for low field $B^2$ region as seen in log-log plots. The Kohler's rule, $\Delta\rho_{xx}(B,T)/\rho_{xx}(0,T) = f(B/\rho_{xx}(0,T))$, holds only for the high field $B$-linear contribution. (E-F) The low field $B^2$-contribution is scaled by $B^2/\rho_{xx}(0,T)$ rather than

$B/\rho_{xx}(0,T)$ at least up to 100 K, indicating the violation of Kohler's rule for the low field $B^2$-contribution. The curve at 200 K does not overlay curves for lower temperatures. This deviation may be attributed to the offset by inelastic scattering very likely phonon contribution which is not observed in crossover behavior in $\rho_{xy}(B)$ in Fig. 2(b).

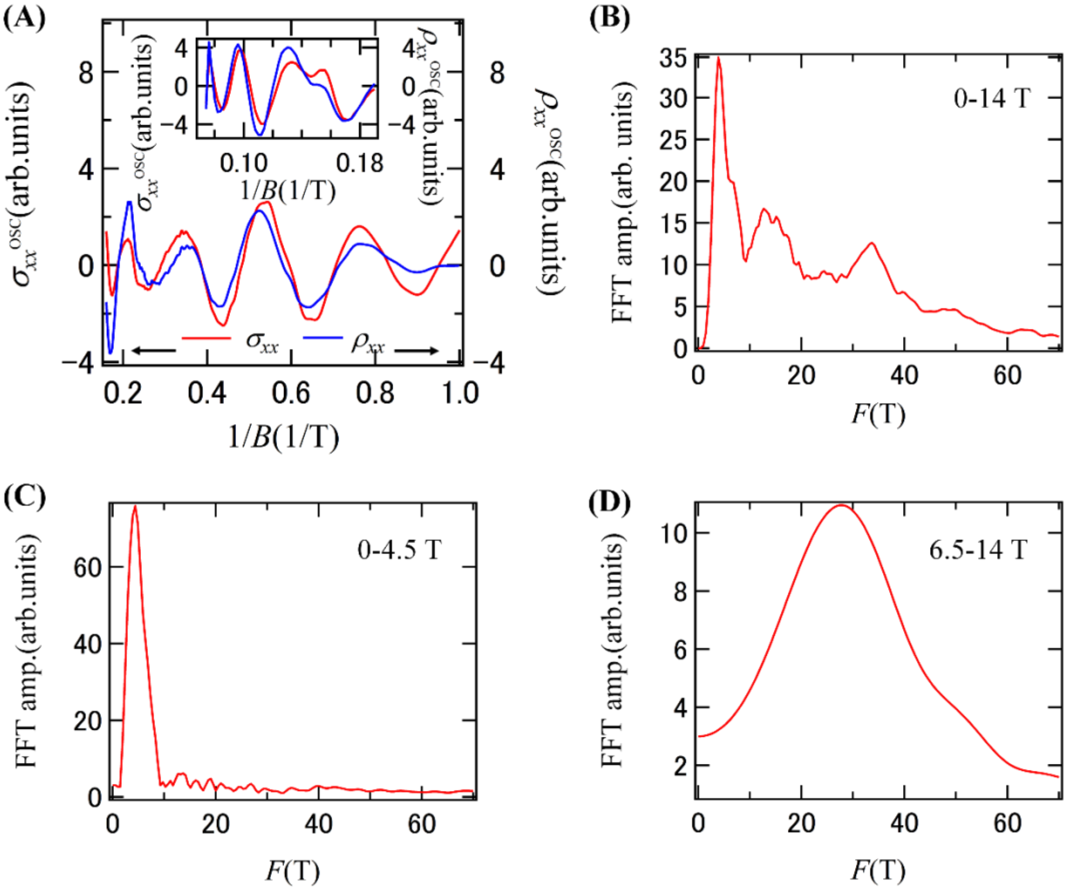


FIG. S5. Further analysis of SdH oscillations.
(A) Comparison of the oscillatory part of $\rho_{xx}(B)$, $\rho_{xx}^{\mathrm{Osc}}(B)$, shown in Fig. 4A and that of $\sigma_{xx}(B)$, $\sigma_{xx}^{\mathrm{Osc}}(B)$, at $T$=2 K. The maxima of $\sigma_{xx}^{\mathrm{Osc}}(B)$ is located at the maxima of $\rho_{xx}^{\mathrm{Osc}}(B)$.
(B-D) FFT spectrum of $\rho_{xx}^{\mathrm{Osc}}$ at 2 K for 0-14 T shows three peaks around ~5 T, ~14 T and ~32 T. The additional broad peak around 14 T is not observed in FFT spectrum for both 0-4.5 T and 6.5-14 T, though the peak around ~32 T in (D) is broad due to a small number of oscillations. This indicates that 14 T peaks is generated by a beating of 5 T and 32 T oscillations, as 14 ~ (32-5)/2.

| | $l_{tot}$ (μm) | $l_c$ (μm) | $w$ (μm) | $t$ (μm) |
|---|---|---|---|---|
| main text | 652 | 271 | 236 | 225 |
| Fig. S1 | 624 | 245 | 245 | 259 |

TABLE S1. The dimensions of the samples used in the main text and FIG. S1. $l_{tot}$, $l_c$, $w$ and $t$ are the total length, the distance between voltage contacts, the width and the thickness, respectively.
